# Supplementary material for: On the Equivalence between Online and Private Learnability beyond Binary Classification
Source: arXiv:2006.01980 source file (2021-10-09)
Supplement: Supplementary file 1 [file appendix.tex]

%!TEX root = main.tex

\section{Appendix}
\wip
